# Supplementary material for: Tunneling spectroscopy of graphene nanodevices coupled to large-gap superconductors
Source: arXiv:1809.09376 source file (2018-09-25)
Supplement: Supplementary file 1 [file N-QD-SG_Supmat_v5_-_light.pdf]

# Supplemental Material for: "Tunneling spectroscopy of graphene nanodevices coupled to large gap superconductors "

Joel I-Jan Wang[1], Landry Bretheau[1,2]*, Daniel Rodan-Legrain[1], Riccardo Pisoni[3], Kenji Watanabe[3], Takashi Taniguchi[3], Pablo Jarillo-Herrero[1]*
[1] Department of Physics, Massachusetts Institute of Technology, 77 Massachusetts Avenue, Cambridge, Massachusetts 02139, United States
[2] Laboratoire des Solides Irradiés, Ecole Polytechnique, CNRS, CEA, 91128 Palaiseau, France
[3] Solid State Physics Laboratory, ETH Zürich, CH-8093 Zürich, Switzerland
[4] National Institute for Materials Science, Namiki 1-1, Tsukuba, Ibaraki 305-0044, Japan
* landry.bretheau@polytechnique.edu

## 1. Device fabrication

The van der Waals heterostructures are assembled using the procedure and recipe reported previously [1], with a few improvements that we describe below:

- The major novelty in the fabrication process consists in a top hBN layer that lies on top of both the graphene flake and the graphite tunneling probe (Fig. 1a in main text). It fully encapsulates the active region of the device in order to reduce the disorder.
- The superconducting leads are connected to the graphene sheet through 1-D edge contacts [2,3]. They are defined by e-beam lithography followed by reactive ion etching that etches the hBN and graphene to expose the graphene edge. The e-beam evaporation of Ti (5 nm) sticking layer, and the reactive sputtering of Nb/NbN (15 nm / 50 nm) are performed in the same chamber with base pressure ~ $8 \times 10^{-9}$ Torr.

Improvement in the device quality is evidenced by the observation of zero *dI/dV* at phase $\varphi = 0$ (Fig. 1e in the main text) and a well-pronounced phase modulation of the ABS around the charge neutrality point (Fig. 2c in the main text).

## 2. Measurement setup

The device is thermally anchored at 20 mK to the mixing chamber of a dilution refrigerator. Differential measurements (*dI/dV* and *dV/dI*) are performed at low (7~30 Hz) frequency using standard lock-in techniques, with excitation $dV \sim 15$ μV and $dI \sim 10$ nA for voltage and current bias measurement respectively. More details about the measurement setup and DC filtering scheme can be found in Ref. [1].

## 3. Differential conductance measurements of graphene in the normal regime

The normal (non-superconducting) graphene density of states can be extracted by measuring the differential conductance *dI/dV* with a DC bias energy much larger than the superconducting gap. Fig. S1 shows such *dI/dV* vs. $V_g$ measurements for tunnel junction #4 (Fig. S1a) and tunnel junction #1 (Fig. S1b). Both junctions exhibit a V-shape dependence with a minimum at the charge neutrality point (CNP), as expected from graphene's linear DOS (Dirac cone). Note that graphene nanodevices measured by tunneling spectroscopy are slightly hole-doped (DOS minimum at the CNP for $V_g$>0), while SGS devices measured by transport are slightly electron-doped (minimum of supercurrent at the CNP for $V_g$<0) (see Fig 1c). We attribute this to two different types of

doping. For SGS junctions, graphene is encapsulated in hBN and is only doped by the superconducting electrodes at its edge, leading to an average electron-doping (non-uniform doping). For tunneling graphene nanodevices, the central region is hole-doped by the graphite probe that is lying just on top of it (separated by a ~nm thick hBN tunnel barrier). Combined with the n-doping of the S edge contacts, it leads to an average hole-doping of the graphene central region.

On top of the V-shaped DOS, narrow and large spikes are observed in *dI/dV*, which correspond to the Coulomb diamond peaks that are discussed in the main text (Fig. 3). They are associated with microscopic quantum dots, with typical charging energy $\sim 5-60$ meV. Their characteristic size $d=\sqrt{C_g/c_g}$ can be inferred from the diamonds' dimension (Fig. 3) knowing the gate capacitance per unit area $c_g \approx 0.1$ fF μm$^{-2}$. Here, $C_g = e/\delta V_g$ is the gate capacitance, with $\delta V_g$ the separation (at $E=0$) between two consecutive diamonds belonging to the same quantum dot. Performing this analysis, we estimate $d \sim 5-20$ nm.

## 4. ABS spectra of other graphene weak links: observation of phase jumps

In the main text, we focused on junction #1 for the phase dependence of graphene DOS in the superconducting regime (see Fig. 2). Similar measurements were performed for junctions #4 and #5, as shown in Fig. S2. Strikingly, the *dI/dV* measurements show abrupt jumps (marked by black arrows on top axes) as the *B*-field is swept. They are visible around zero magnetic field and disappear at larger field. These phase jumps are all the more present as the graphene weak link is wide ($W=2.7$ μm for junction #4 and $W=3.4$ μm for junction #5), and are absent in junction #1, which is the narrowest of our junctions ($W=1.3$ μm).

We believe this phenomenon is associated with how the superconducting phase is distributed along the superconducting loop:

- When the Josephson inductance $L_J$ of the graphene weak link is much larger than the inductance of the Nb/NbN loop $L_{Nb/NbN}$, all the phase difference $\varphi=\phi/\phi_0=\varphi_G$ drops across graphene. In this case, the phase difference across graphene $\varphi_G$ is directly proportional to the magnetic flux $\phi$ (and field $B$). This happens for "large" $L_J$ / "small" Josephson current $I_J$ and therefore narrow graphene.
- But when the graphene weak link is wider, the loop inductance $L_{Nb/NbN}$ is no longer negligible compared to the graphene Josephson inductance $L_J$. Then, part of the global phase difference $\varphi$ drops along the Nb/NbN loop, and $\varphi_G \neq \varphi$. Since $L_J$ depends on $\varphi_G$, this phenomenon leads to abrupt jumps of $\varphi_G$ and therefore of the measured DOS while the magnetic field is swept.
- At large enough field, the Josephson current $I_J$ is reduced due to magnetic flux penetrating graphene and dephasing of the ABS (Fraunhofer interference). Therefore $L_J$ is increased and dominates $L_{Nb/NbN}$ and the phase jumps disappear.

These phase jumps prevent from measuring accurately the ABS spectra. The observation of this phase jump regime might be facilitated by the use of a large gap superconductor.

## 5. Tunneling spectroscopy of the S-G-S junctions in the Fraunhofer regime

With our device (Fig. 1b), one can measure the differential conductance $dI/dV$ (and therefore the DOS) in the weak link between tunnel junction #3 and #4, which is not enclosed on a superconducting loop. By applying a magnetic field $B$, a magnetic flux $\phi = B * A$ penetrates the graphene area $A$, which affects the superconducting proximity effect. This is what is shown in Fig. S3, where $dI/dV$ is plotted as a function of both energy $E = eV$ and the reduced flux $2\pi\phi/\phi_0$ (this is not the superconducting phase difference across the junction, which remains zero here in the absence of a loop). We observe that $dI/dV$ modulates with magnetic field with a periodicity corresponding to the flux quantum. The visibility of the oscillations decreases with the magnetic field and can be seen up to $2\pi\phi/\phi_0 \sim 3$ ($B \sim 3.5$ mT). The induced gap is maximally decreased each time an additional flux quantum threads the graphene area. This is a direct spectroscopic observation of the Fraunhofer interference as Josephson vortices start to form in the graphene rectangular weak link [4].

## 6. Tunneling spectroscopy and supercurrent measurements at large magnetic field

Using Nb/NbN contacts allows one to perform both tunneling and transport measurements at magnetic field higher than what is accessible with aluminum-based devices. Fig. S4a shows the $dI/dV$ measurement of junction #1 up to $B$=15 mT, corresponding to more than 10 magnetic flux quanta penetrating the graphene area. We observe that the phase modulation of the graphene DOS around the induced superconducting gap remain visible in this entire range, with a decreasing visibility as the $B$-field increases.

We also perform transport measurement of graphene Josephson weak links under high magnetic field. The encapsulated S-G-S junctions (not presented in the main text) employ the same metallization recipe as the tunneling devices. Fig. S4b plots the $dV/dI$ measurement at $V_g$ = -0.81 V in the Fraunhofer regime up to $B$=2 mT. We observe that the oscillatory behavior of the critical current $I_c$ deviates from the conventional Fraunhofer pattern, denoted by the red curve superimposed on the data, and shows irregularities in the periodicities and amplitude of $I_c$. This departure from the conventional Fraunhofer pattern could be related to the existence of ABS that form near graphene edge, as recently observed in Ref. [5].

Finally, we plot in Fig. S4c the 2-D color map of $dV/dI$ measured with respect to $V_g$ and $B$-field up to 5 T. The white curve superimposed on the data highlights the semi-classical limit $L = 2 * r_c$, where $r_c$ is the cyclotron radius. When $L/2 \le r_c$ (low magnetic fields), zero resistance is observed demonstrating the good proximity effect. Note that the superconductivity is suppressed more rapidly by increasing the B-field for hole-dope region, which results from the p-n interfaces given by the contact n-doping [1,5]. When $L/2 > r_c$, although ABS should not be able to form in the bulk, we still observe random pockets of close to zero resistance regions [5,6]. This phenomenon however disappears when entering in the quantum Hall regime, where the Landau fan is clearly visible.

Therefore, although we did not observe the existence of supercurrent carrying states in the quantum Hall regime [6], we observed that the superconducting proximity effect

survives in large magnetic fields (up to $B \sim 1$ T). This could be related to unconventional ABS that survive near the graphene edges [5].


[1] L. Bretheau, J. I-Jan Wang, R. Pisoni, K. Watanabe, T. Taniguchi, and P. Jarillo-Herrero, Nat. Phys. **13**, 756-760 (2017).

[2] L. Wang, I. Meric, P. Y. Huang, Q. Gao, Y. Gao, H. Tran, T. Taniguchi, K. Watanabe, L. M. Campos, D. A. Muller, J. Guo, P. Kim, J. Hone, K. L. Shepard, and C. R. Dean, Science **342**, 614-617 (2013).

[3] V. E. Calado, S. Goswami, G. Nanda, M. Diez, A. R. Akhmerov, K. Watanabe, T. Taniguchi, T. M. Klapwijk, and L. M. K. Vandersypen, Nat. Nanotechnol. **10**, 761-764 (2015).

[4] D. Roditchev, C. Brun, L. Serrier-Garcia, J. C. Cuevas, V. H. L. Bessa, M. V. Milošević, F. Debontridder, V. Stolyarov, and T. Cren, Nat. Phys. **11**, 332-337 (2015).

[5] M. Ben Shalom, M. J. Zhu, V. I. Fal'ko, A. Mishchenko, A. V. Kretinin, K. S. Novoselov, C. R. Woods, K. Watanabe, T. Taniguchi, A. K. Geim, and J. R. Prance, Nat. Phys. 12, 318-322 (2015).

[6] F. Amet, C. T. Ke, I. V. Borzenets, J. Wang, K. Watanabe, T. Taniguchi, R. S. Deacon, M. Yamamoto, Y. Bomze, S. Tarucha, and G. Finkelstein, Science **352**, 966-969 (2016).

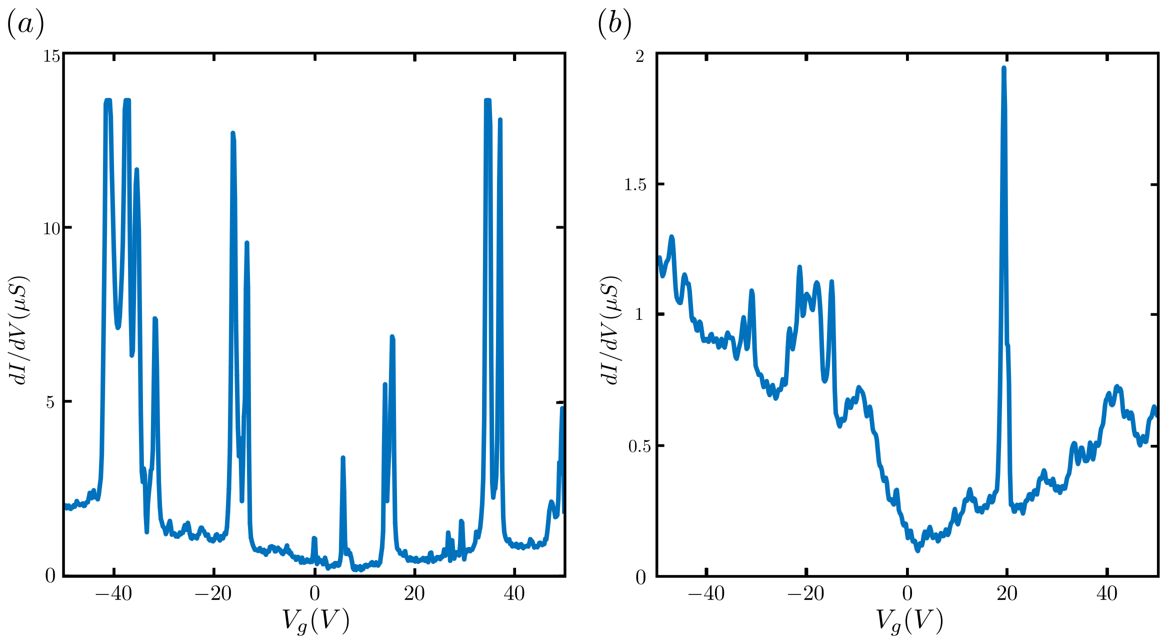


**Figure S1. Graphene DOS in the normal state.** Differential conductance, *dI/dV*, measured as a function of backgate voltage $V_g$ in tunnel junction #4 **(a)** and #1 **(b)**. The overall V-shape feature of the *dI/dV* is related to the linear dispersion of graphene DOS. Giant spikes observed in both measurements are associated with the Coulomb blockade diamonds and originate from microscopic quantum dots.

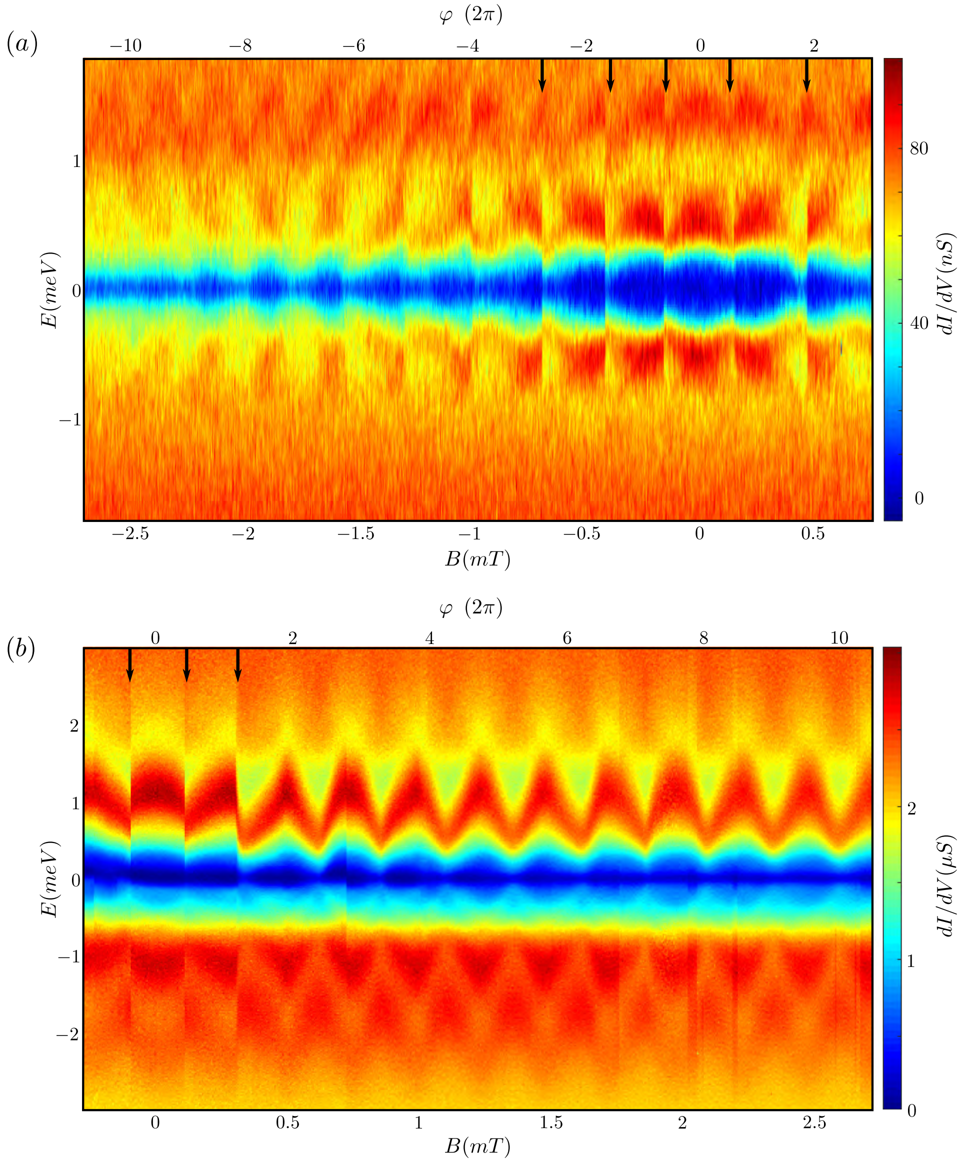


**Figure S2. Phase jumps in the ABS spectra.** Color-coded *dI/dV* versus energy *E*=*eV* and magnetic field *B* (lower axis) and φ (top axis) measured in tunnel junction #4 **(a)** and #5 **(b)**. Black arrows on top of each panel point to the locations where the jumps occur. These jumps disappear as |B| increases.

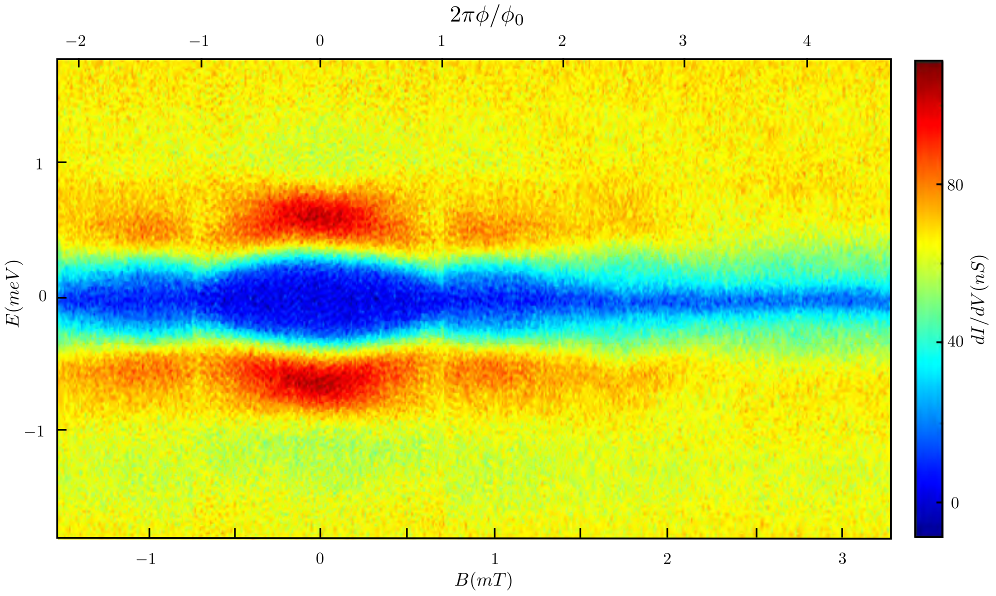


**Figure S3. Tunneling spectroscopy of the S-G-S junction in the Fraunhofer regime.** *dI/dV* measurement taken as a function of energy $E$ and magnetic field $B$ (the top axis shows $B$ converted into the reduced magnetic flux $2\pi\phi/\phi_0$ penetrating the graphene area). The oscillatory behavior of the induced gap is reminiscent from the Fraunhofer pattern observed in the supercurrent of Josephson junctions under magnetic field.

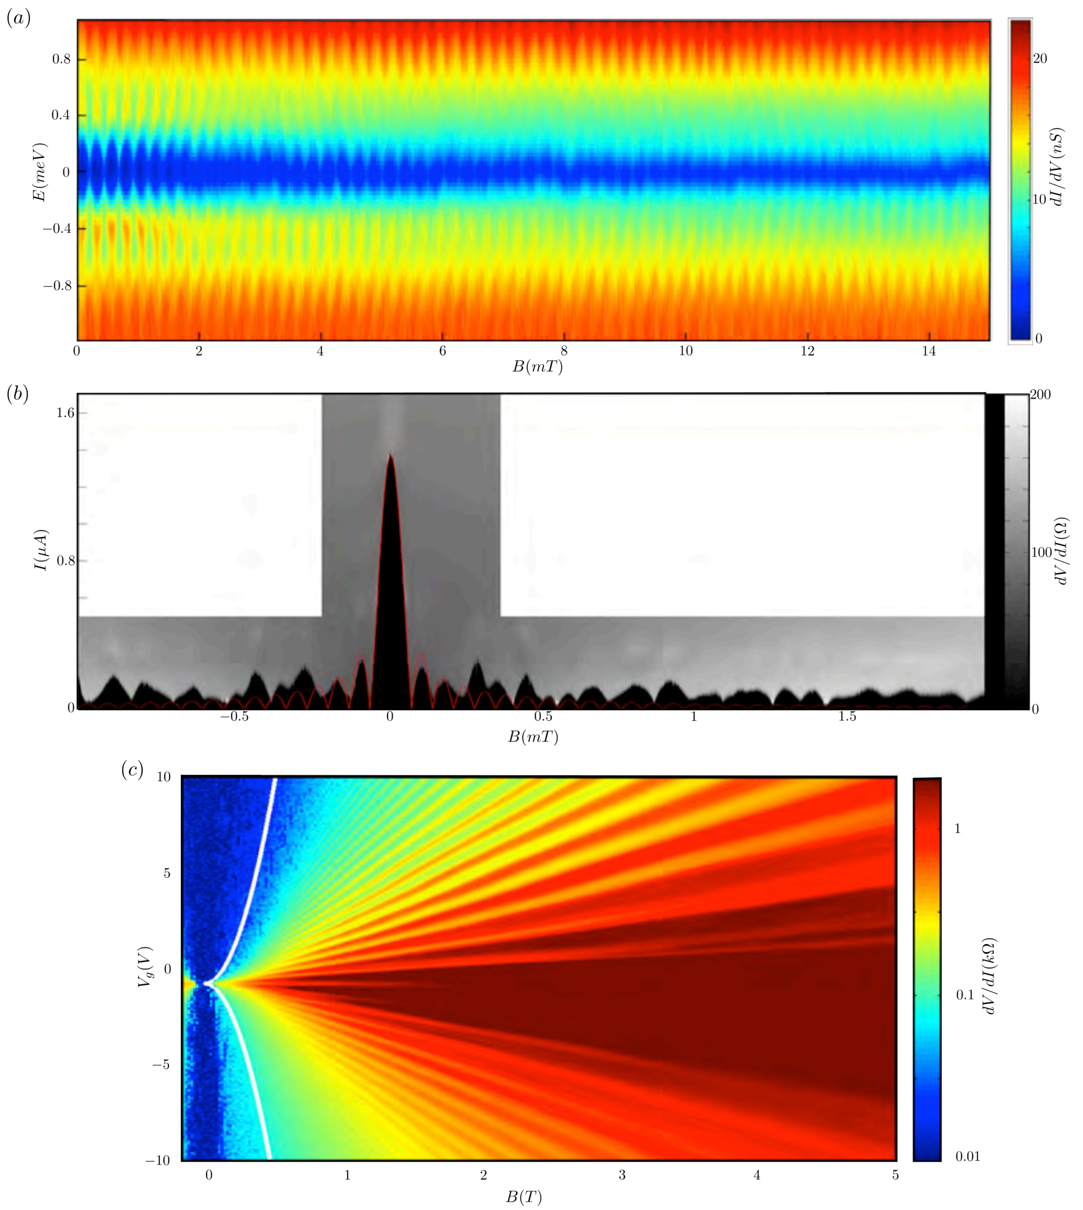


**Figure S4. Characterization at high magnetic field. (a)** *dI/dV* measurement of tunnel junction #1 as a function of both energy and magnetic field, up to $B$=15 mT. The phase modulation of the ABS remains robust even though the graphene accommodates more than 10 magnetic flux quanta in it (1 flux quantum quantum corresponds here to ~1.3 mT). **(b)** Differential resistance, *dV/dI,* of a SGS junction measured as a function of bias current $I$ and magnetic field $B$. The oscillatory behavior of the maximum supercurrent, defined by the onset of finite resistance, exhibits a clear departure from the conventional Fraunhofer pattern (highlighted by the red curve). **(c)** *dV/dI* of a SGS junction measured as a function of magnetic field $B$ and gate voltage $V_g$. The white curve denotes the semi-classical limit $L/2=R_c$, where $R_c$ is the cyclotron radius. For *n*-doping ($V_g>V_{CNP}$ ~ -0.8 V), the junction exhibits superconductivity at low field until the cyclotron radius becomes comparable to the junction length. Immediately beyond this limit, one still observes randomly distributed pockets of ~ zero resistance until the Landau fan pattern dominates the diagram. In the *p*-doping region, the superconductivity is suppressed more strongly by increasing $B$-field due to the *p*-*n* interface given by the *n*-doping from the metal contacts.
